# Supplementary material for: Model-based Smoothing with Integrated Wiener Processes and Overlapping Splines
Source: arXiv:2302.02053 source file (2023-02-04)
Supplement: Supplementary file 1 [file Appendix_of_Smoothing_Project.pdf]

# 1 Appendix A: Derivation with Finite Element Method

The Finite Element Method (FEM) can be understood as the following procedures.

Given a stochastic differential equation (SDE)  $Dg(t) = \xi(t)$ , where  $D$  is a linear differential operator and  $\xi(t)$  is a known generalized GP [3] such as the Gaussian white noise process. The region of interest  $\Omega$  is assumed to be a bounded interval on  $\mathbb{R}$ . Let  $\mathbb{B}_k := \{\varphi_i, i \in [k]\}$  denote the set of  $k$  pre-specified basis functions, and let  $\mathbb{T}_q := \{\phi_i, i \in [q]\}$  denote the set of  $q$  pre-specified test functions. We consider an finite dimensional approximation  $\tilde{g}(\cdot)$  to the true function  $g(\cdot)$ , defined as:

$$\tilde{g}(\cdot) = \sum_{i=1}^k w_i \varphi_i(\cdot), \quad (1)$$

where  $\mathbf{w} := (w_1, \dots, w_k)^T \in \mathbb{R}^k$  is a set of random weights to be determined.

To determine the unknown weight vector  $\mathbf{w}$ , we seek the weak solution of the SDE relative to the test functions  $\mathbb{T}_q$ , that is:

$$\langle D\tilde{g}(t), \phi_i(t) \rangle_{\Omega} \stackrel{d}{=} \langle \xi(t), \phi_i(t) \rangle_{\Omega}, \quad (2)$$

for any test function  $\phi_i \in \mathbb{T}_q$ . This equation 2 implicitly defines the distribution on the  $k$ -dimensional weight vector, which will be multivariate Gaussian with precision matrix structure depending on the choice of  $\mathbb{T}_q$  and  $\mathbb{B}_k$ . Specifically, the inner products  $\langle D\tilde{g}(t), \phi_i(t) \rangle_{i=1}^q$  can be vectorized as

$$\langle D\tilde{g}(t), \phi_i(t) \rangle_{i=1}^q = H\mathbf{w},$$

where the  $ij$  component of the  $q \times k$   $H$  matrix can be computed as

$$H_{ij} = \langle D\varphi_j(t), \phi_i(t) \rangle.$$

The second inner products  $\langle \xi(t), \phi_i(t) \rangle_{i=1}^q$  will have Gaussian distribution with zero mean vector and  $q \times q$  covariance matrix  $B$  determined by the choice of  $\xi(t)$  and  $\mathbb{T}_q$ . When the generalized GP  $\xi(t)$  is the standard Gaussian white noise process, the covariance matrix  $B$  has element  $B_{ij} = \langle \phi_i(t), \phi_j(t) \rangle$  [2].

To derive the proposed O-spline approximation, we use the piece-wise constant test functions  $\mathbb{T}_k := \{\phi_i, i \in [k]\}$  and  $p$ th order O-spline basis  $\mathbb{B}_k := \{\varphi_i, i \in [k]\}$ , defined over the same set of knots  $\mathbf{s} = \{s_i : i \in [k]\} \subset \Omega$ :

$$\phi_i(t) = \begin{cases} 0 & \text{if } t < s_{i-1}, \\ 1 & \text{if } t \in (s_{i-1}, s_i], \\ 0 & \text{if } t \geq s_i. \end{cases}, \quad \varphi_i(t) = \begin{cases} 0 & \text{if } t < s_{i-1}, \\ \frac{(t-s_{i-1})^p}{p!} & \text{if } t \in (s_{i-1}, s_i], \\ \sum_{k=1}^p \frac{d_i^k (t-s_i)^{p-k}}{k!(p-k)!} & \text{if } t \geq s_i. \end{cases} \quad (3)$$

where  $d_i := s_i - s_{i-1}$ .

By definition of O-spline basis, we have  $D\varphi_i(t) := \frac{\partial^p \varphi_i}{\partial t^p}(t) = \phi_i(t)$ . This basis and test space construction is called least square solution [3]. With this choice of test/basis function, the matrix  $B$  satisfies:

$$B_{ij} = \langle \phi_i(t), \phi_j(t) \rangle = \langle D\varphi_j(t), \phi_i(t) \rangle = H_{ij}.$$

Therefore equation 2 implies  $\mathbf{w} \sim N(0, B^{-1})$ , where  $B$  is diagonal with  $i$ th diagonal element being  $\langle \phi_i(t), \phi_i(t) \rangle$ .

## 2 Appendix B: Proof Of Main Theorems

**Theorem 1** (Convergence of Overlapping spline). *Let  $\Omega = [a, b]$  where  $a, b \in \mathbb{R}^+$  and let  $f \sim IWP_{0-p}$  with  $p \geq 1$  being any positive integer. Assume the knots  $\{s_1, \dots, s_k\}$  are equally spaced over  $\Omega$  for each  $k \in \mathbb{N}$ , and  $\tilde{f}_k(x)$  denotes the corresponding  $p$ th order overlapping spline (O-spline) approximation, then:*

$$\lim_{k \rightarrow \infty} \sup_{s, t \in \Omega} |\mathcal{C}(s, t) - \mathcal{C}_k(s, t)| = 0,$$

where  $\mathcal{C}(s, t) = \text{Cov}[f(s), f(t)]$  and  $\mathcal{C}_k(s, t) = \text{Cov}[\tilde{f}_k(s), \tilde{f}_k(t)]$ .

*Proof.* To prove this theorem to general integer order  $p$ , we will start with the case when  $p = 1$ . Assume without the loss of generality that  $\Omega = [0, 1]$  and hence  $s_i = i/k$  for each  $i$ . Then the true covariance function of IWP in this case will be

$$\mathcal{C}(s, t) = \min\{s, t\}.$$

To compute the covariance of the approximation, we have the following:

$$\begin{aligned} \mathcal{C}_k(s, t) &:= \text{Cov}\left(\tilde{f}_k(s), \tilde{f}_k(t)\right) \\ &= \text{Cov}\left(\sum_{i=1}^k w_i \varphi_i(s), \sum_{i=1}^k w_i \varphi_i(t)\right) \\ &= k \Phi(s)^T \Phi(t), \end{aligned} \tag{4}$$

where  $\Phi(t) = (\varphi_1(t), \dots, \varphi_k(t))^T$  and  $\Phi(s) = (\varphi_1(s), \dots, \varphi_k(s))^T$ , because of the distribution of  $w_i \stackrel{iid}{\sim} N(0, k)$  according to our definition.

Now assume that  $s \leq t$  without loss of generality. Because of the overlapping property of the O spline basis  $\varphi_i$ , it is obvious that only knots located in the region  $[0, s]$  will have basis functions with non-trivial contribution to the above inner product. Therefore,

$$\begin{aligned} k \Phi(s)^T \Phi(t) &= k \sum_{i=1}^{\lfloor ks \rfloor} \varphi_i(s) \varphi_i(t) \\ &= k \sum_{i=1}^{\lfloor ks \rfloor} \frac{1}{k^2} \text{ since } p = 1 \\ &= \lfloor ks \rfloor / k, \end{aligned} \tag{5}$$

since  $\phi_i(s) = \phi_i(t) = \frac{1}{k}$  for  $i \leq \lfloor ks \rfloor$ .

For any fixed  $t \in \Omega$ , we have

$$\begin{aligned} \sup_{s \in \Omega} |\mathcal{C}(s, t) - \mathcal{C}_k(s, t)| &\leq \sup_{s \in [0, t]} |\mathcal{C}(s, t) - \mathcal{C}_k(s, t)| + \sup_{s \in [t, 1]} |\mathcal{C}(s, t) - \mathcal{C}_k(s, t)| \\ &= \sup_{s \in [0, t]} |s - \lfloor ks \rfloor / k| + \sup_{s \in [t, 1]} |t - \lfloor kt \rfloor / k| \\ &\leq 2/k. \end{aligned} \tag{6}$$

Since  $t$  is arbitrary, this implies  $\sup_{s,t \in \Omega} |\mathcal{C}(s,t) - \mathcal{C}_k(s,t)| \leq 2/k$  and hence we prove the case for  $p = 1$ .

To generalize the result to higher order of  $p$ , we need the following lemma about Gaussian process:

**Lemma 1** (Integration of Gaussian Process). *Assume  $f(t)$  is Gaussian process with continuous sample path for  $t \in \Omega := [0, 1]$  with the boundary condition  $f(0) = 0$ , then  $g(s) := \int_0^s f(t)dt$  is still a Gaussian process, and its covariance function at  $s^*, t^* \in \Omega$  can be computed as*

$$\mathcal{C}_g(s^*, t^*) = \int_0^{s^*} \int_0^{t^*} \mathcal{C}_f(s, t) dt ds$$

where  $\mathcal{C}_f(\cdot)$  is the covariance function of  $f$ .

This lemma follows from section 2.4.3 of [1].

Now, consider the case where  $p = 2$ , then because of the derivative consistency property of the overlapping spline basis, it is immediate that  $\frac{\partial \tilde{f}(x)}{\partial x}$  is the first order O spline approximation for the first order IWP  $\frac{\partial f(x)}{\partial x}$ , whose convergence is already established in the proof above. Furthermore for  $p = 1$ , the proposed approximation has continuous sample path and covariance function  $\mathcal{C}_k(s, t) = \lfloor ks \rfloor / k \leq 1$  as shown above.

Let  $\mathcal{C}^{[p]}(s, t)$  and  $\mathcal{C}_k^{[p]}(s, t)$  denote the covariance of the  $p$ th order IWP and its approximation, then for any choice of  $s, t \in \Omega$ , we have:

$$\begin{aligned} & \sup_{s,t \in \Omega} |\mathcal{C}^{[2]}(s, t) - \mathcal{C}_k^{[2]}(s, t)| \\ &= \sup_{s,t \in \Omega} \left| \int_0^s \int_0^t \mathcal{C}^{[1]}(s^*, t^*) - \mathcal{C}_k^{[1]}(s^*, t^*) dt^* ds^* \right| \\ &\leq \sup_{s,t \in \Omega} \int_0^s \int_0^t \left| \mathcal{C}^{[1]}(s^*, t^*) - \mathcal{C}_k^{[1]}(s^*, t^*) \right| dt^* ds^* \\ &\leq \sup_{s,t \in \Omega} \int_0^1 \int_0^1 \left| \mathcal{C}^{[1]}(s^*, t^*) - \mathcal{C}_k^{[1]}(s^*, t^*) \right| dt^* ds^* \\ &\leq \int_0^1 \int_0^1 \frac{2}{k} dt^* ds^* \text{ by previous result on } p = 1 \\ &= \frac{2}{k}. \end{aligned} \tag{7}$$

So the convergence of covariance function for  $p = 2$  is established. Furthermore, because the region  $[0, s] \times [0, t] \subseteq \Omega \times \Omega$  is compact, the covariance function for higher order  $p$  will still be bounded by  $2/k$ . Hence the convergence result can be generalized to any positive integer  $p$  by induction.  $\square$

**Theorem 2** (Convergence of Cross-Covariance). *Let  $\Omega = [a, b]$  where  $a, b \in \mathbb{R}^+$  and let  $p \geq 1$  and  $q \leq p - 1$  be arbitrary positive integers. Let  $f \sim \text{IWP}_{0-p}$ .*

Assume the knots  $\{s_1, \dots, s_k\}$  are equally spaced over  $\Omega$  for each  $k \in \mathbb{N}$ , and  $\tilde{f}_k(x)$  denotes the corresponding  $p$ th order ( $O$ -spline) approximation, then:

$$\lim_{k \rightarrow \infty} \sup_{s, t \in \Omega} |\mathcal{C}^{(0,q)}(s, t) - \mathcal{C}_k^{(0,q)}(s, t)| = 0,$$

where  $\mathcal{C}^{(0,q)}(s, t) = \text{Cov}[f(s), f^{(q)}(t)]$  and  $\mathcal{C}_k^{(0,q)}(s, t) = \text{Cov}[\tilde{f}_k(s), \tilde{f}_k^{(q)}(t)]$ .

*Proof.* For the ease of notation, define the differentiation and integration operators as

$$D_t^p(g(s, t)) := \frac{\partial^p g}{\partial t^p}(s, t),$$

and

$$I_t^p(g(s, t)) := \int_0^t \int_0^{t_1} \dots \int_0^{t_{p-1}} g(s, t_p) dt_p dt_{p-1} \dots dt_1.$$

Both operators are linear. Again for simplicity we consider  $\Omega = [0, 1]$  without the loss of generality. When  $p = 1$  the theorem is trivial, so we consider the case where  $p > 1$ .

Let  $s, t \in \Omega$  be fixed and let  $f$  follows the  $p$ th order IWP with  $\tilde{f}_k$  denotes its approximation. Let  $\mathcal{C}^{[p]}(s, t)$  denotes its auto-covariance and  $\mathcal{C}_k^{[p]}(s, t)$  denotes the auto-covariance of the approximation.

Following from the proof of theorem 1,  $\{\mathcal{C}_k^{[p]}(s, t)\}_k$  are uniformly bounded. Applying the Fubini's theorem with result of lemma 1, we get:

$$\begin{aligned} \mathcal{C}_k^{(0,q)}(s, t) &= \mathbb{E}[\tilde{f}_k(s) \frac{\partial^q}{\partial t^q} \tilde{f}_k(t)] \\ &= \frac{\partial^q}{\partial t^q} \mathbb{E}[\tilde{f}_k(s) \tilde{f}_k(t)] \\ &= D_t^q \mathcal{C}_k^{[p]}(s, t) \\ &= D_t^q I_t^{p-1} I_s^{p-1} [\mathcal{C}_k^{[1]}(s, t)] \\ &= I_t^{p-q-1} I_s^{p-1} [\mathcal{C}_k^{[1]}(s, t)]. \end{aligned} \tag{8}$$

Similarly,  $\mathcal{C}^{(0,q)}(s, t)$  can be written as:

$$\begin{aligned} \mathcal{C}^{(0,q)}(s, t) &= D_t^q \mathcal{C}^{[q]}(s, t) \\ &= I_t^{p-q-1} I_s^{p-1} [\mathcal{C}^{[1]}(s, t)]. \end{aligned} \tag{9}$$

Then the following upper bound can be achieved with the result of theorem 1:

$$\begin{aligned} \sup_{s, t \in \Omega} |\mathcal{C}^{(0,q)}(s, t) - \mathcal{C}_k^{(0,q)}(s, t)| &= \sup_{s, t \in \Omega} |I_t^{p-q-1} I_s^{p-1} \mathcal{C}^{[1]}(s, t) - \mathcal{C}_k^{[1]}(s, t)| \\ &\leq \sup_{s, t \in \Omega} I_t^{p-q-1} I_s^{p-1} |\mathcal{C}^{[1]}(s, t) - \mathcal{C}_k^{[1]}(s, t)| \\ &\leq \sup_{s, t \in \Omega} I_t^{p-q-1} I_s^{p-1} \frac{2}{k} \\ &\leq \frac{2}{k}, \end{aligned} \tag{10}$$

where the last inequality follows from the compactness of  $\Omega$ .

□

## References

- [1] Robert J Adler. *The geometry of random fields*. SIAM, 2010.
- [2] Andrew C Harvey. Forecasting, structural time series models and the kalman filter. 1990.
- [3] Finn Lindgren, Havard Rue, and Johan Lindstrom. An explicit link between gaussian fields and gaussian markov random fields: the stochastic partial differential equation approach. *Journal of the Royal Statistical Society, Series B (Statistical Methodology)*, 73(4):423–498, 2011.
